# Supplementary material for: A Concurrent Unbounded Wait-Free Graph
Source: arXiv:1810.13325 source file (2019-04-24)
Supplement: Supplementary file 1 [file appendix.tex]

\begin{center}
\Large\textbf{Appendix}
\end{center}
\label{sec:appendix}
\section{\FPSP}
\label{sec:app-fpsp}
